# Supplementary material for: CARLA Drone: Monocular 3D Object Detection from a Different Perspective
Source: arXiv:2408.11958 source file (2024-10-21)
Supplement: Supplementary file 6 [file supp_groundmix_imgs.tex]

\begin{figure}[t]
\centering
%\begin{tabular}{l r}
\minipage{0.13\textwidth}
\includegraphics[width=\textwidth]{figures/supp_groundmix1.png}
\endminipage \,
\minipage{0.13\textwidth}
\includegraphics[width=\textwidth]{figures/supp_groundmix2.pdf}
\endminipage \,
\minipage{0.13\textwidth}
\includesvg[width=\textwidth]{figures/supp_groundmix3.svg}
\endminipage \,
\minipage{0.13\textwidth}
\includegraphics[width=\textwidth]{figures/supp_groundmix4.png}
\endminipage \,
\minipage{0.13\textwidth}
\includegraphics[width=\textwidth]{figures/supp_groundmix5.png}
\endminipage\hfill
%\end{tabular}
\caption{\textbf{Soft pasting in comparison with pasting of Mix-Teaching \cite{main-mix-teaching}. } \textbf{Image 1:} The patch to be pasted. \textbf{Image 2:} Sampling of the mask ($a_1, a_2 \in [0, 10\%\cdot A]$, $b_1, b_2 \in [0, 20\%\cdot B]$) \textbf{Image 3:} The corresponding mask, where black denotes 0\% opacity and white denotes 100\% opacity. \textbf{Image 4:} Result after pasting the object softly with the mask of image 3. \textbf{Image 5:} Pasting as done in Mix-Teaching \cite{main-mix-teaching}. In contrast to Mix-Teaching \cite{main-mix-teaching}, our approach does not provide the network hints about the 2D bounding box .} 
\label{tab:patch_pasting}
\end{figure}
